# Supplementary material for: Reproducibility and Evolution of Diffusion MRI Measurements within the Cervical Spinal Cord in Multiple Sclerosis
Source: arXiv:2108.03575 source file (2021-08-08)
Supplement: Supplementary file 1 [file figures_suplementaires.tex]

\documentclass{llncs}
\usepackage{graphicx}
\usepackage{placeins}
\usepackage{float}
\usepackage{subfigure}

\begin{document}

\begin{figure}[H] 
  \includegraphics[width=0.99\textwidth]{miccai_figures/exolain_pralel_figures.jpg}
  
  \caption{how we compute Bland altman and how plot difference between basline and M12}
\end{figure}

\begin{figure}[H] 
  \includegraphics[width=0.99\textwidth]{miccai_figures/numero_de_patients.jpg}
  
  \caption{Patients ID for various evolution}
\end{figure}

\section{figures}
\begin{figure}[H] 
  \includegraphics[width=0.62\textwidth]{miccai_figures/altman/g-dti-altman-dti_ad.png}
  \includegraphics[width=0.62\textwidth]{miccai_figures/altman/g-dti-altman-dti_fa.png}
  \caption{altman-dti ad for controls-----altman-dti fa for controls}
\end{figure}

\begin{figure}[H] 
  \includegraphics[width=0.62\textwidth]{miccai_figures/altman/g-dti-altman-dti_rd.png}
  \includegraphics[width=0.62\textwidth]{miccai_figures/altman/g-dti-altman-dti_md.png}
  \caption{altman-dti rd for controls-----altman-dti md for controls}
\end{figure}

\begin{figure}[H] 
  \includegraphics[width=0.62\textwidth]{miccai_figures/altman/g-dti-altman-stick_ad.png}
  \caption{altman- STICK ad}
\end{figure}

\begin{figure}[H] 
  \includegraphics[width=0.62\textwidth]{miccai_figures/altman/g-dti-altman-ball_weights.png}
  \includegraphics[width=0.62\textwidth]{miccai_figures/altman/g-dti-altman-stick_weights.png}
  \caption{altman-ball and stick weights of controls}
\end{figure}

\subsection{Paralell plot}

\begin{figure}[H] 
  \includegraphics[width=0.62\textwidth]{miccai_figures/patientDiffM0M12/g-dti-paralellplotdti_ad.png}
  \includegraphics[width=0.62\textwidth]{miccai_figures/patientDiffM0M12/g-dti-paralellplotdti_fa.png}
  \caption{Difference between M0 and M12 for AD and FA for controls}
\end{figure}

\begin{figure}[H] 
  \includegraphics[width=0.62\textwidth]{miccai_figures/patientDiffM0M12/g-dti-paralellplotdti_rd.png}
  \includegraphics[width=0.62\textwidth]{miccai_figures/patientDiffM0M12/g-dti-paralellplotdti_md.png}
  \caption{Difference between M0 and M12 for RD and MD for controls}
\end{figure}

\begin{figure}[H] 
  \includegraphics[width=0.62\textwidth]{miccai_figures/patientDiffM0M12/g-dti-paralellplotstick_ad.png}
  \caption{Difference between M0 and M12 for ID for controls}
\end{figure}

\begin{figure}[H] 
  \includegraphics[width=0.62\textwidth]{miccai_figures/patientDiffM0M12/g-dti-paralellplotball_weights.png}
  \includegraphics[width=0.62\textwidth]{miccai_figures/patientDiffM0M12/g-dti-paralellplotstick_weights.png}
  \caption{Difference between M0 and M12 for ball and stick weights for controls}
\end{figure}

\subsection{cmpCtlPatM0}

\begin{figure}[H] 
  \includegraphics[width=0.62\textwidth]{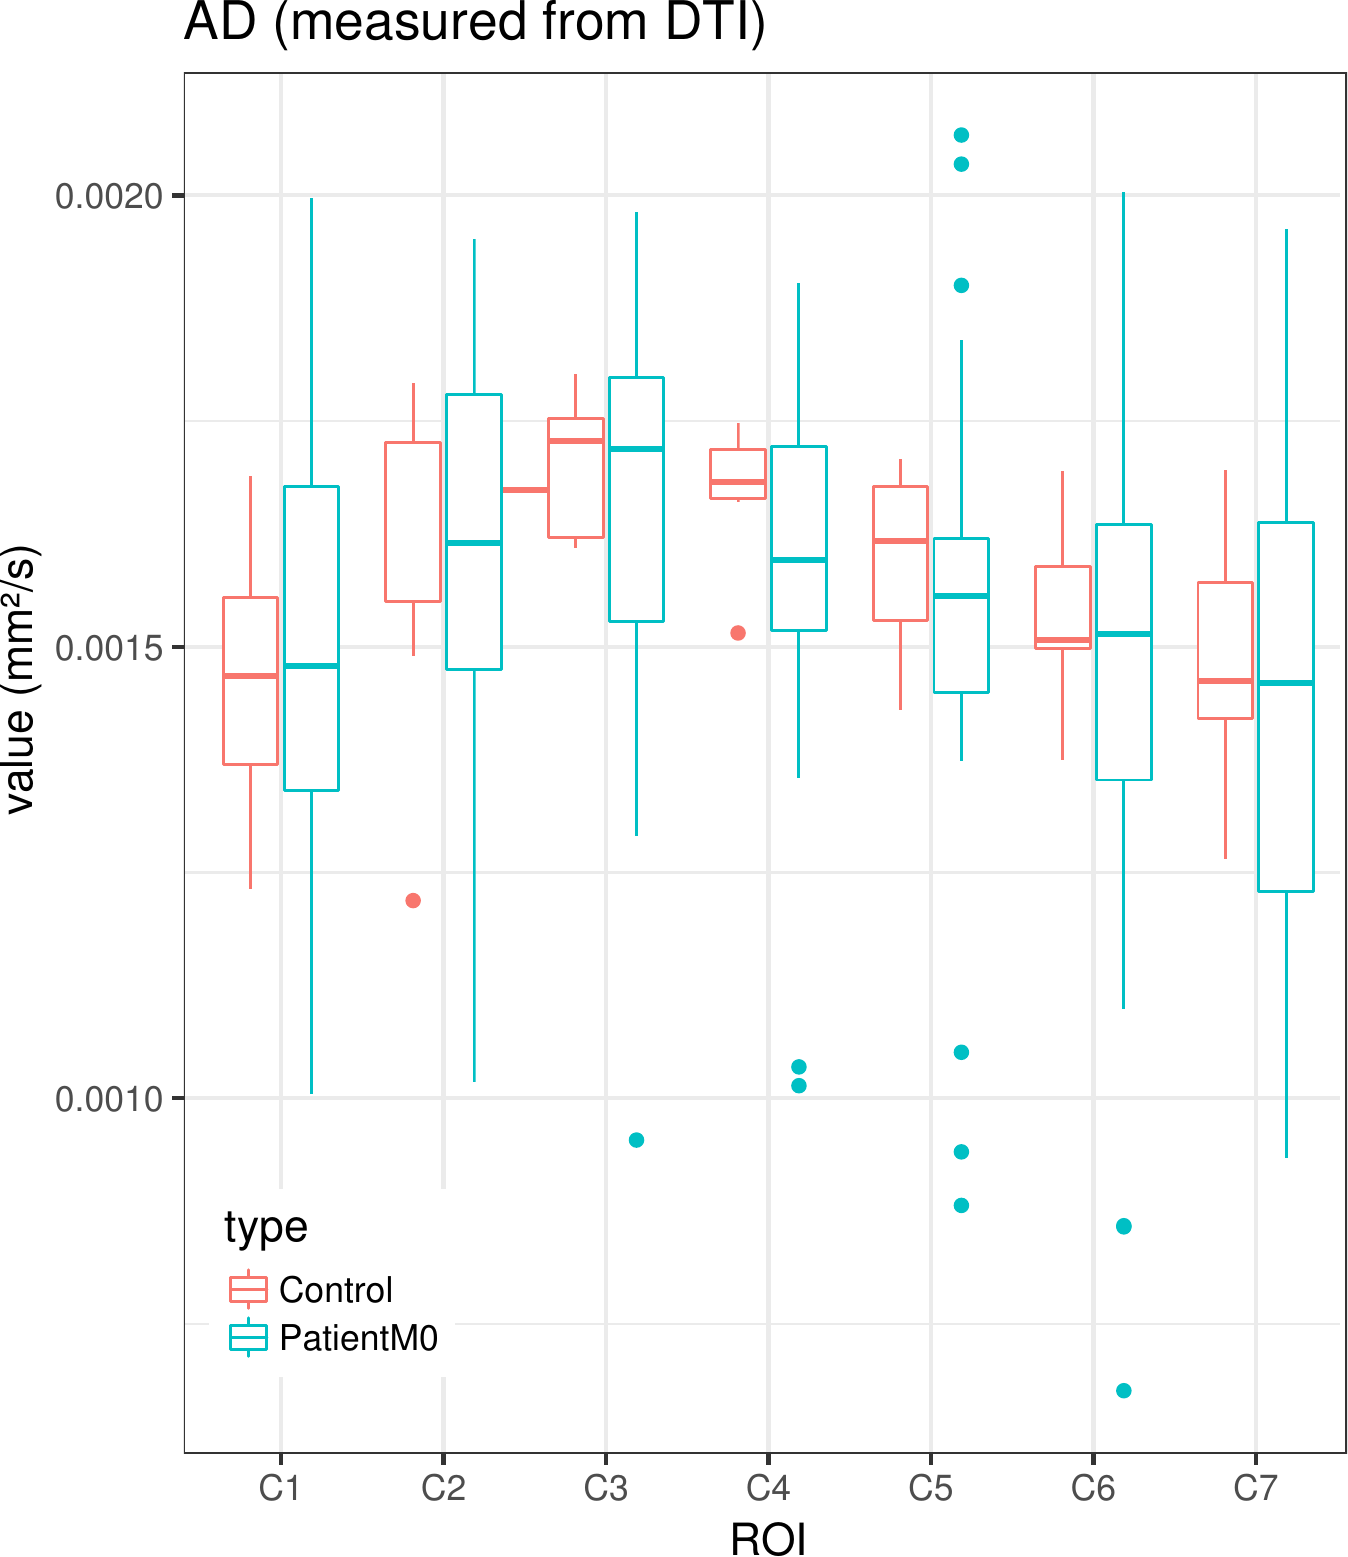}
  \includegraphics[width=0.62\textwidth]{miccai_figures/cmpCtlPatM0/miccai18-cmp-dti_fa.png}
  \caption{boxplot of AD and FA for controls}
\end{figure}

\begin{figure}[H] 
  \includegraphics[width=0.62\textwidth]{miccai_figures/cmpCtlPatM0/miccai18-cmp-dti_rd.png}
  \includegraphics[width=0.62\textwidth]{miccai_figures/cmpCtlPatM0/miccai18-cmp-dti_md.png}
  \caption{boxplot of RD and MD for controls}
\end{figure}

\begin{figure}[H] 
  \includegraphics[width=0.62\textwidth]{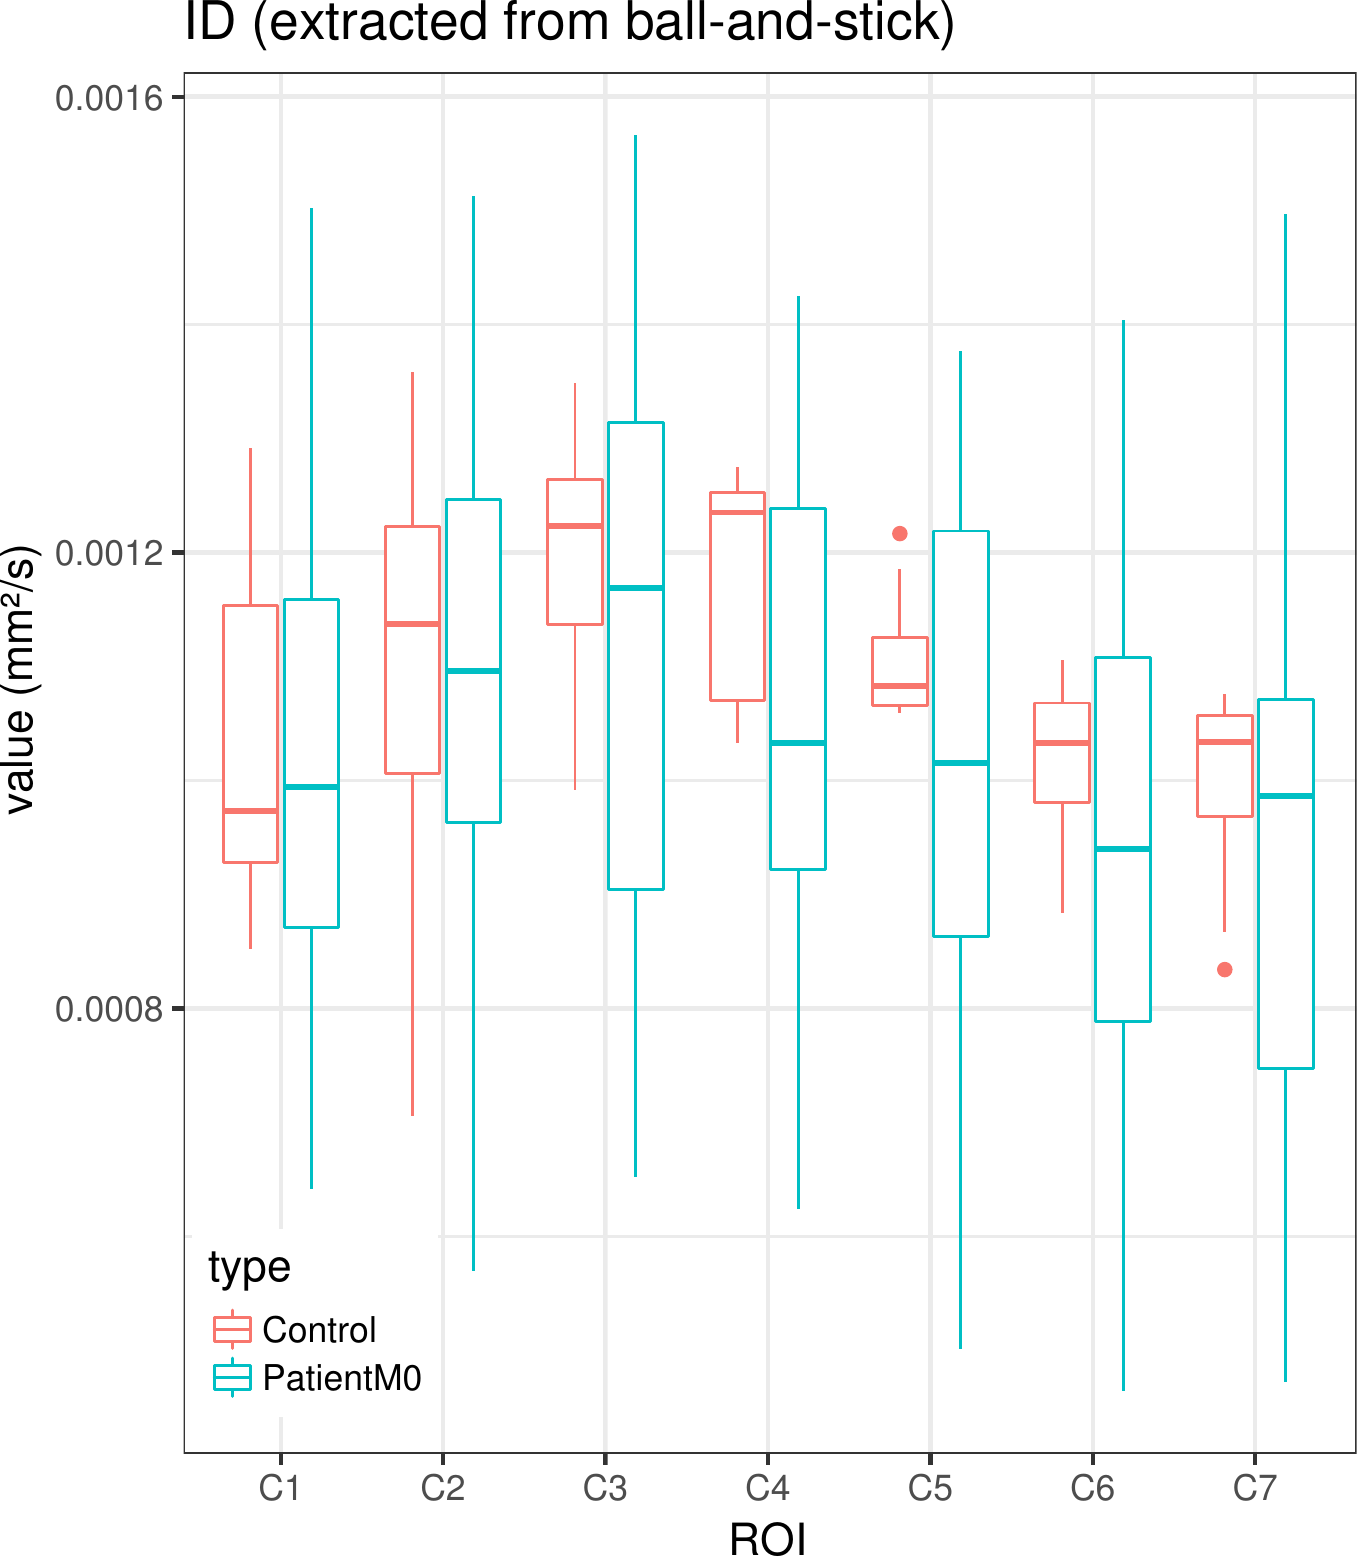}
  \caption{boxplot of ID}
\end{figure}

\begin{figure}[H] 
  \includegraphics[width=0.62\textwidth]{miccai_figures/cmpCtlPatM0/miccai18-cmp-ball_weights.png}
  \includegraphics[width=0.62\textwidth]{miccai_figures/cmpCtlPatM0/miccai18-cmp-stick_weights.png}
  \caption{boxplot of ball and stick weights of controls}
\end{figure}

\end{document}
